# Supplementary material for: Improving DRAM Performance, Reliability, and Security by Rigorously Understanding Intrinsic DRAM Operation
Source: arXiv:2303.07445 source file (2023-03-13)
Supplement: Supplementary file 1 [file changelog.tex]

\chapter{Changelog}

\begin{itemize}
    \item v1.4 --- 2021-09-27 --- Miscellaneous writing polishing throughout Sections 2.3.4 and Chapter 7.
    \item v1.3 --- 2021-09-15 --- General writing improvements throughout Sections 2.3.4 and 7.1-7.4.
    \item v1.2 --- 2021-09-13 --- Added the fourth row to Table 7.1.
    \item v1.1 --- 2021-09-13 --- Writing clarifications to Sections 2.3.4, 7.2, and 7.3.
    \item v1.0 --- 2021-09-11 --- Initial release.
\end{itemize}
